# Supplementary material for: Archetypal soft-mode driven antipolar transition in francisite Cu3Bi(SeO3)2O2Cl
Source: arXiv:1907.12069 ancillary file (2019-12-19)
Supplement: Supplementary file 1 [file Soft_mode_in_francisite___Supplement.pdf]

Supplemental Material

Cosme Milesi-Brault,<sup>1,2</sup> Constance Toulouse,<sup>2</sup> Evan Constable,<sup>3</sup> Hugo Aramberri,<sup>1</sup> Virginie Simonet,<sup>4</sup> Sophie de Brion,<sup>4</sup> Helmuth Berger,<sup>5</sup> Luigi Paolasini,<sup>6</sup> Alexei Bosak,<sup>6</sup> Jorge Íñiguez,<sup>1,2</sup> and Mael Guennou<sup>2</sup>

<sup>1</sup>Materials Research and Technology Department,

Luxembourg Institute of Science and Technology, 41 rue du Brill, L-4422 Belvaux, Luxembourg

<sup>2</sup>University of Luxembourg, Physics and Materials Science Research Unit, 41 rue du Brill, L-4422 Belvaux, Luxembourg

<sup>3</sup>Institute of Solid State Physics, Vienna University of Technology, 1040 Vienna, Austria

<sup>4</sup>Université Grenoble Alpes, CNRS, Institut Néel, 38000 Grenoble, France

<sup>5</sup>Institute of Physics of Complex Matter, École Polytechnique Fédérale de Lausanne, CH-1015 Lausanne, Switzerland

<sup>6</sup>European Synchrotron Radiation Facility, BP 220, F-38043 Grenoble Cedex, France

(Dated: July 28, 2019)

I. PHONON DISPERSION BY INELASTIC X-RAY SCATTERING

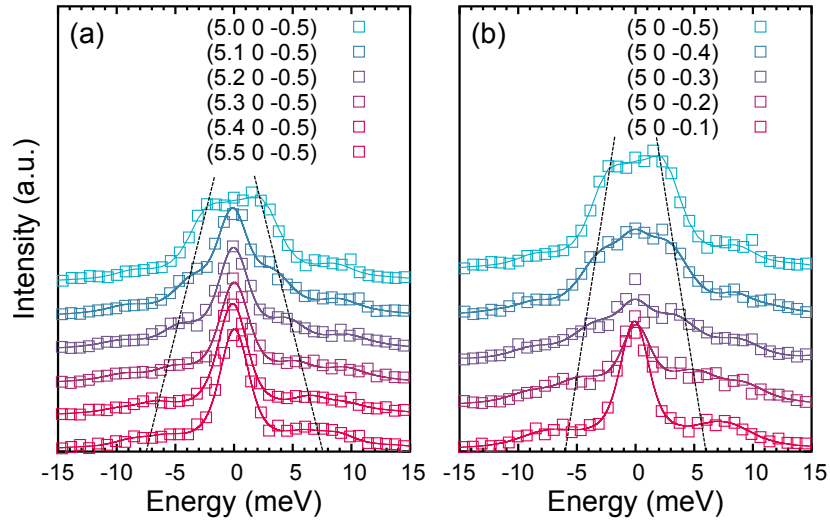

Figure 1: Dispersion (a) along the  $h$  direction and (b) along the  $l$  direction measured at room temperature. The solid line is the result from the fit and the dotted line is a guide for the eye following the soft mode.

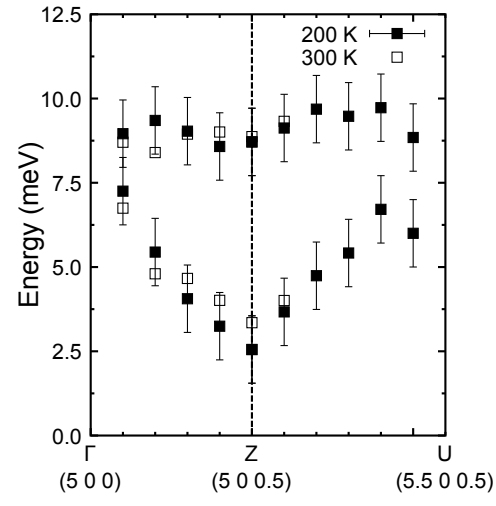

Figure 2: Dispersion along the  $\Gamma$ -Z-U path at 200 and 300 K measured by Inelastic X-Ray Scattering.

## II. CALCULATION DETAILS

The calculations were carried out within the Density Functional Theory framework as implemented in the VASP code, using the Perdew-Burke-Ernzerhof approximation to the exchange-correlation functional. The strong electronic correlations were taken into account within the GGA+U approach. The Coulomb repulsion was set to  $U=9.5$  eV for the d orbitals of Cu, while the exchange coupling was set to  $J=1.0$  eV. We employed a plane-wave energy cutoff 500 eV for the basis set in all our calculations. A  $3 \times 2 \times 3$  ( $3 \times 2 \times 1$ )  $k$ -mesh was used in the calculations of the  $Pm\bar{m}n$  ( $Pcmn$ ) primitive cell. Atoms were allowed to relax until atomic forces became smaller than  $0.01$  eV/Å. The phonon dispersions were calculated using the frozen-phonon approach in 120-atom supercells ( $2 \times 1 \times 2$ ) supercells with respect to the  $Pm\bar{m}n$  primitive cell).

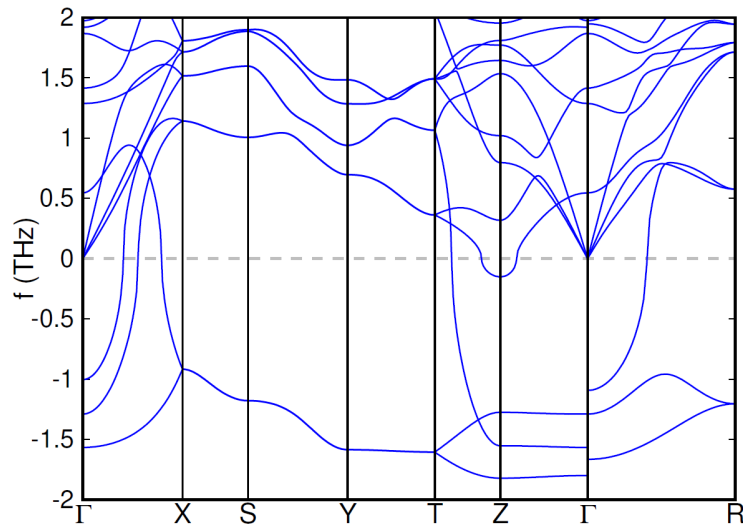

Figure 3: Phonon dispersion of Francisite in the high symmetry phase ( $Pm\bar{m}n$ ) as computed in its primitive cell.

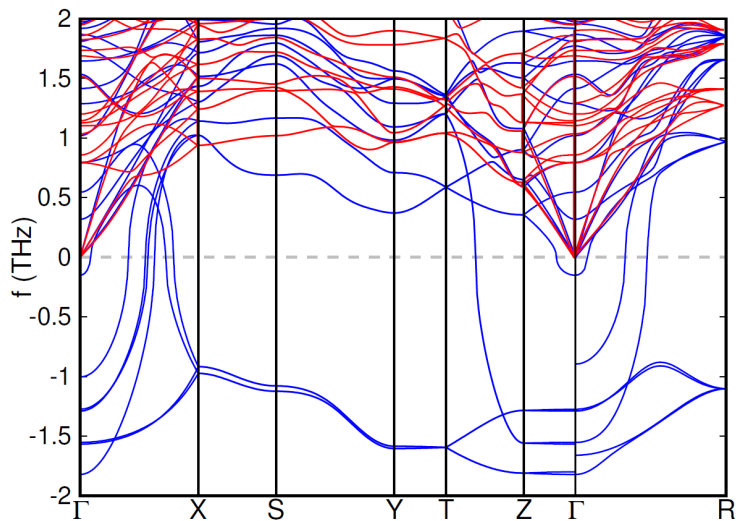

Figure 4: Phonon dispersion of Francisite in the high symmetry phase (blue) and low symmetry (red) phases. The former has now been computed in a  $1 \times 1 \times 2$  supercell with respect to its primitive cell, so that it can be compared to the phonons of the low symmetry phase. Note that the Z point of the primitive cell of the  $Pm\bar{m}n$  phase is folded onto the  $\Gamma$  point of the supercell shown here. Thus, the antipolar mode in the primitive Z point is now at the  $\Gamma$  point slightly below the ferroelectric mode. The low symmetry phase shows no unstable modes.
